# Supplementary material for: Smoke and Mirrors in Causal Downstream Tasks
Source: arXiv:2405.17151 source file (2025-02-10)
Supplement: Supplementary file 1 [file prerequisites.tex]

\section{Prerequisites}
\label{sec:prerequisites}
